# Supplementary material for: Drawing the LINE: Cryptographic Analysis and Security Improvements for the LINE E2EE Protocol
Source: arXiv:2602.18370 source file (2026-02-20)
Supplement: Supplementary file 1 [file SM_security.tex]

\fbox{
\begin{minipage}{0.22\textwidth}
\hspace{0.25cm}
    \underline{$\initO$}
    \begin{algorithmic}[1]
    \State $\key \getsr \KeySpace$
    \State $\state_A \gets \initA(\key)$ 
    \State $\state_A \gets \initA(\key)$ 
    \State $(\epoch_A,\epoch_B) \gets (0,0)$ 
    \State $\indexsm_A,\indexsm_B \gets 0$ 
    \State $\epoch_L \gets -\infty$ 
    \State $\trans, \chall, \comp \gets \emptyset$ 
    \State $b \tor \bits$  
    \end{algorithmic}        

%%%%%%%%%%%%%%%%%%%%%%%%%%%%%%%%%%%%%%%%%%%%%%%%%%%%%%%%%%%%%
\hspace{0.25cm}
    \underline{$\corrA$}
    \begin{algorithmic}[1]
    \State $\req ~B \not\in \chall$
    \If {$\compS = true$}
    \State $\comp \getplus \trans(B)$
    \State $\epoch_L \gets max(\epoch_A, \epoch_B)$
    \EndIf
    \State \Return $\state_A$
    \end{algorithmic} 

%%%%%%%%%%%%%%%%%%%%%%%%%%%%%%%%%%%%%%%%%%%%%%%%%%%%%%%%
\hspace{0.25cm}
    \underline{$\transmitA(\msg,\random)$}
    \begin{algorithmic}[1]
    \State $(\random,\flag) \gets \SamIfNec(\random)$
    \State $\epmgmt (A,\flag)$
    \State $\indexsm_A++$
    \State $(\state_A,\ciphertxt) \gets \send(\state_A,\msg;\random)$
    \State $\record(A,norm,\msg,\ciphertxt)$
    \State \Return $\ciphertxt$
    \end{algorithmic} 
%%%%%%%%%%%%%%%%%%%%%%%%%%%%%%%%%%%%%%%%%%%%%%%%%%%%%%%%%
\hspace{0.25cm}
    \underline{$\challA(\msg_0,\msg_1,\random)$}
    \begin{algorithmic}[1]
    \State $(\random,\flag) \gets \SamIfNec(\random)$ 
    \State $\epmgmt(A,\flag)$
    \State $\req \safech_A ~and |\msg_0| = |\msg_1|$ 
    \State $\indexsm_A ++$
    \State $(\state_A,\ciphertxt) \gets \send(\msg_b;\random)$
    \State $\record(A,\chall,\msg_b,\ciphertxt)$
    \State \Return $\ciphertxt$
    \end{algorithmic}

%%%%%%%%%%%%%%%%%%%%%%%%%%%%%%%%%%%%%%%%%%%%%%%%%%%%%%%%%
\hspace{0.25cm}
    \underline{$\deliverA(\ciphertxt)$}
    \begin{algorithmic}[1]
    \State$ \req (B,\epoch,\indexsm,\msg,\ciphertxt) \in \trans$
    \State $for ~some ~\epoch,\indexsm,\msg$
    \State $(\state_A,\epoch',\indexsm',\msg') \gets \Rcv(\state_A,\ciphertxt) $
    \If{$(\epoch',\indexsm',\msg') \neq (\epoch,\indexsm,\msg)$}
    \State $\win$
    \If{$(\epoch,\indexsm,\msg) \in \chall$}
    \State $\msg' \gets \bot$
    \EndIf
    \EndIf
    \State $\epoch_A \gets max(\epoch_A,\epoch_B)$
    \State $\delete(\epoch,\indexsm)$
    \State \Return $(\epoch',\indexsm',\msg')$
    \end{algorithmic}
    \end{minipage}
\vline

%%%%%%%%%%%%%%%%%%%%%%%%%%%%%%%%%%%%%%%%%%%%%%%%%%%%%%%%%
\begin{minipage}{0.22\textwidth}
\hspace{0.25cm}
    \underline{$\injectA(\ciphertxt)$}
    \begin{algorithmic}[1]
    \State $\req ~ (B,\ciphertxt) \not\in \trans~and~\safeinj$
    \State $(\state_A,\epoch',\indexsm',\msg') \gets \Rcv(\state_A,\ciphertxt)$ 
    \If{$\msg' \neq \bot ~and ~(B,\epoch',\indexsm') \not\in \comp$}
    \State $\win$
    \EndIf
    \State $\epoch_A \gets max(\epoch_A,\epoch')$ 
    \State $\delete (\epoch',\indexsm')$
    \State \Return $(\epoch',\indexsm',\msg')$
    \end{algorithmic}

%%%%%%%%%%%%%%%%%%%%%%%%%%%%%%%%%%%%%%%%%%%%%%%%%%%%%%%%%
\hspace{0.25cm}
    \underline{$\epmgmt(P,\flag)$}
    \begin{algorithmic}[1]
    \If{$P = A ~and ~\epoch_P~even ~or P = B ~and \epoch_P ~odd$}
    \If {$\flag = bad ~and \urcorner \safech_P$}
    \State $\epoch_L \gets \epoch_P +1$
    \EndIf
    \EndIf
    \State $\epoch_P++$
    \State $\indexsm_P \gets 0$
    \end{algorithmic}

%%%%%%%%%%%%%%%%%%%%%%%%%%%%%%%%%%%%%%%%%%%%%%%%%%%%%%
\hspace{0.25cm}
    \underline{$\SamIfNec(\random)$}
    \begin{algorithmic}[1]
    \State $\flag \gets bad$
    \If{$\random = \bot$}
    \State $\random \getsr \RandomSpace$
    \State $\flag \gets good$ 
    \EndIf
    \State \Return $(\random,\flag)$
    \end{algorithmic}

%%%%%%%%%%%%%%%%%%%%%%%%%%%%%%%%%%%%%%%%%%%%%%%%%%%%%%
\hspace{0.25cm}
    \underline{$\record(P,\flag,\msg,\ciphertxt)$}
    \begin{algorithmic}[1]
    \State $\rec \gets (P,\epoch_P,\indexsm_P,\msg,\ciphertxt)$
    \State $\trans \getplus \rec$
    \If{$\urcorner \safech_P$}
    \State $\comp \getplus \rec$
    \EndIf
    \If{$\flag = \chall$}
    \State $\chall \getplus \rec$  
    \EndIf
    \end{algorithmic}

%%%%%%%%%%%%%%%%%%%%%%%%%%%%%%%%%%%%%%%%%%%%%%%%%%
\hspace{0.25cm}
\underline{$\delete(\epoch,\indexsm)$}
    \begin{algorithmic}[1]
    \State $\rec \gets (P,\epoch,\indexsm_P,\msg,\ciphertxt)$ 
    \State $for ~some ~P,\msg,\ciphertxt$ 
    \State $\trans,\chall,\comp \getminus \rec$
    \State $\safech_P :\Longleftrightarrow \epoch_p \geq \epoch_L + \Delta_{\SM}$
    \State $\safeinj :\Longleftrightarrow min(\epoch_A,\epoch_B) \geq \epoch_L +$ 
    \State $\Delta_{\SM}$
    \end{algorithmic}
   \vspace{0.5cm}
 \end{minipage}
}
